# Supplementary material for: Bayesian Approaches to Designing Replication Studies
Source: arXiv:2211.02552 source file (2023-08-11)
Supplement: Supplementary file 1 [file batdrs-supplement.pdf]

# Bayesian Approaches to Designing Replication Studies Supplementary Materials

**Samuel Pawel*, Guido Consonni†, Leonhard Held***
* Department of Biostatistics, University of Zurich
† Dipartimento di Scienze Statistiche, Università Cattolica del Sacro Cuore
E-mail: samuel.pawel@uzh.ch

August 11, 2023

In this document we provide additional information on computing the predictive distribution of the replication effect estimate when a prior is assigned to the heterogeneity variance $\tau^2$ (Section 1). We also provide additional information on methods for analyzing replication data. For each method we derive the *success region* in terms of the effect estimate of the replication study $\hat{\theta}_r$, which is required for sample size determination as illustrated in the main manuscript (Section 2 to 7). For the two-trials rule and the replication Bayes factor methods we additionally provide derivations on how these methods can be generalized to the multisite replication setting. We show then how the optimal number of samples per site can be derived for multisite SSD (Section 8). Finally, we show SSD for all studies from the Protzko et al. (2020) project using either a flat prior or an adaptive shrinkage prior for the effect size (Section 9).

## 1 Prior on the heterogeneity variance

When also a prior is assigned to the heterogeneity variance $\tau^2$, the predictive distribution of the replication effect estimate $\hat{\theta}_r$ is given by

$$f(\hat{\theta}_r \mid \hat{\theta}_o, \sigma_o, \sigma_r) = \int_0^{+\infty} f(\hat{\theta}_r \mid \sigma_r, \hat{\theta}_o, \sigma_o, \tau^2)\, f(\tau^2 \mid \hat{\theta}_o, \sigma_o)\, \mathrm{d}\tau^2.$$

That is, it is the predictive distribution of the replication effect estimate $\hat{\theta}_r$ integrated with respect to the marginal posterior of $\tau^2$ based on the original data $x_o = \{\hat{\theta}_o, \sigma_o^2\}$. If the initial prior for $\theta$ is normal $\theta \sim \mathrm{N}(\mu_\theta, \sigma_\theta^2)$, and the initial prior for $\tau^2$ has density $f(\tau^2)$, we have

$$\begin{aligned}
f(\tau^2 \mid \hat{\theta}_o, \sigma_o) &= \int_{-\infty}^{+\infty} f(\theta, \tau^2 \mid \hat{\theta}_o, \sigma_o)\, \mathrm{d}\theta \\
&= \frac{\int_{-\infty}^{+\infty} f(\hat{\theta}_o \mid \theta, \tau^2, \sigma_o^2)\, f(\theta \mid \tau^2)\, f(\tau^2)\, \mathrm{d}\theta}{\int_0^{+\infty}\int_{-\infty}^{+\infty} f(\hat{\theta}_o \mid \theta_*, \tau_*^2, \sigma_o^2)\, f(\theta_* \mid \tau_*^2)\, f(\tau_*^2)\, \mathrm{d}\theta_*\, \mathrm{d}\tau_*^2} \\
&= \frac{f(\tau^2)\int_{-\infty}^{+\infty} \mathrm{N}(\hat{\theta}_o \mid \theta, \tau^2 + \sigma_o^2)\ \mathrm{N}(\theta \mid \mu_\theta, \sigma_\theta^2)\, \mathrm{d}\theta}{\int_0^{+\infty} f(\tau_*^2)\int_{-\infty}^{+\infty} \mathrm{N}(\hat{\theta}_o \mid \theta_*, \tau_*^2 + \sigma_o^2)\ \mathrm{N}(\theta_* \mid \mu_\theta, \sigma_\theta^2)\, \mathrm{d}\theta_*\, \mathrm{d}\tau_*^2} \\
&= \frac{f(\tau^2)\ \mathrm{N}(\hat{\theta}_o \mid \mu_\theta, \tau^2 + \sigma_o^2 + \sigma_\theta^2)}{\int_0^{+\infty} f(\tau_*^2)\, \mathrm{N}(\hat{\theta}_o \mid \mu_\theta, \tau_*^2 + \sigma_o^2 + \sigma_\theta^2)\, \mathrm{d}\tau_*^2}.
\end{aligned}$$

To compute the marginal posterior density of $\tau^2$ one numerical integration is hence required. The updating of the prior depends on the distance between prior mean $\mu_\theta$ and the original effect estimate $\hat{\theta}_o$ relative to the prior variance $\sigma_\theta^2$ and the squared standard error $\sigma_o^2$. If an improper uniform prior is assigned to $\theta$

$(\sigma_\theta^2 \to \infty)$, the posterior reduces to the prior

$$\begin{aligned}\lim_{\sigma_\theta^2 \to \infty} f(\tau^2 \mid \hat{\theta}_o, \sigma_o) &= \lim_{\sigma_\theta^2 \to \infty} \frac{f(\tau^2)\, \mathrm{N}(\hat{\theta}_o \mid \mu_\theta, \tau^2 + \sigma_o^2 + \sigma_\theta^2)}{\int_0^{+\infty} f(\tau_*^2)\, \mathrm{N}(\hat{\theta}_o \mid \mu_\theta, \tau_*^2 + \sigma_o^2 + \sigma_\theta^2)\, \mathrm{d}\tau_*^2} \\ &= \lim_{\sigma_\theta^2 \to \infty} \int_0^{+\infty} \frac{f(\tau^2)}{f(\tau_*^2)} \underbrace{\sqrt{\frac{\tau_*^2 + \sigma_o^2 + \sigma_\theta^2}{\tau^2 + \sigma_o^2 + \sigma_\theta^2}}}_{\to 1} \exp\left[-\frac{1}{2}\left\{\underbrace{\frac{(\hat{\theta}_o - \mu_\theta)^2}{\tau^2 + \sigma_o^2 + \sigma_\theta^2}}_{\downarrow 0} - \underbrace{\frac{(\hat{\theta}_o - \mu_\theta)^2}{\tau_*^2 + \sigma_o^2 + \sigma_\theta^2}}_{\downarrow 0}\right\}\right] \mathrm{d}\tau_*^2 \\ &= f(\tau^2).\end{aligned}$$

This means that with a uniform prior nothing can be learned about the variance $\tau^2$ which intuitively makes sense as estimation of a variance requires at least two observations. The phenomenon is illustrated in Figure 1 for the data from the "Labels"experiment (Protzko et al., 2020) as also used in the main manuscript. We see that as the prior standard deviation increases (making the prior more uniform), the marginal posterior density becomes closer to the prior density.

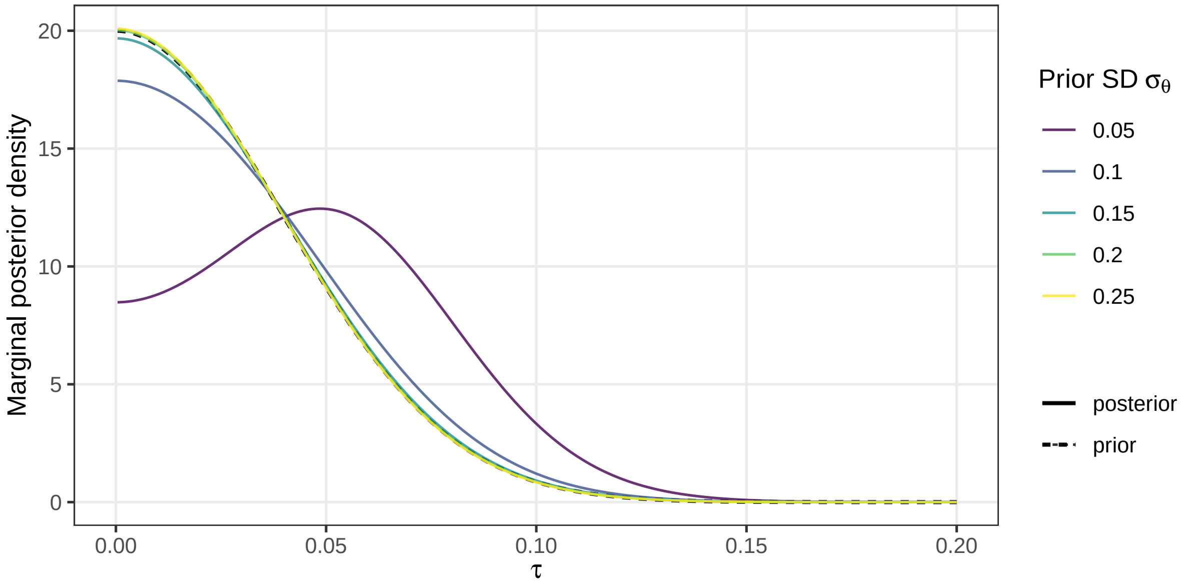


**Figure 1:** Marginal posterior distribution of heterogeneity variance $\tau^2$ based on data from "Labels" experiment (Protzko et al., 2020) with original effect estimate $\hat{\theta}_o = 0.205$ and standard error $\sigma_o = 0.051$. A $\theta \sim \mathrm{N}(0, \sigma_\theta^2)$ prior is assigned to the effect size $\theta$ and a half normal prior with standard deviation $0.04$ is assigned to $\tau$.

Combining all the previous results, we obtain the probability of replication success as

$$\begin{aligned}\Pr(\hat{\theta}_r \in S \mid \hat{\theta}_o, \sigma_o, \sigma_r) &= \int_S \int_0^{+\infty} f(\hat{\theta}_r \mid \hat{\theta}_o, \sigma_o, \sigma_r, \tau^2)\, f(\tau^2 \mid \hat{\theta}_o, \sigma_o)\, \mathrm{d}\hat{\theta}_r\, \mathrm{d}\tau^2 \\ &= \int_0^{+\infty} \Pr(\hat{\theta}_r \in S \mid \hat{\theta}_o, \sigma_o, \sigma_r, \tau^2)\, f(\tau^2 \mid \hat{\theta}_o, \sigma_o)\, \mathrm{d}\tau^2.\end{aligned}$$

This means computing the probability of replication success with a prior on $\tau^2$ requires two-dimensional numerical integration. However, in the common case when a uniform prior is assigned to $\theta$, the marginal posterior distribution of $\tau^2$ reduces to the prior, and only one numerical integration is required.

Figure 2 shows the probability of replication success based on data from the "Labels" experiment,

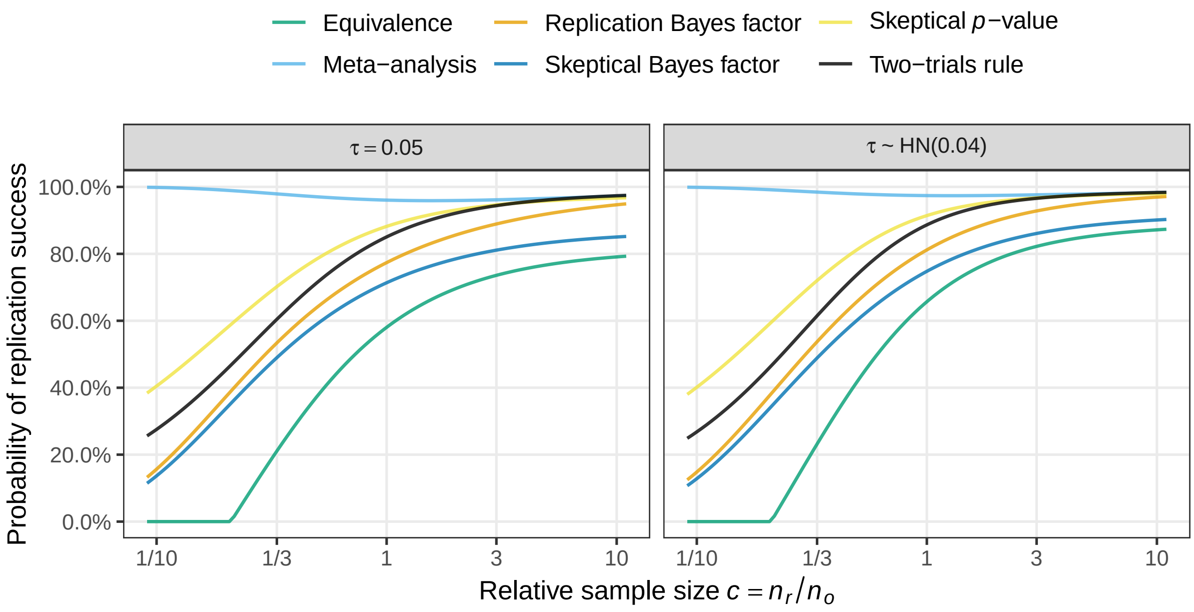


**Figure 2:** Probability of replication success as a function of the relative sample size $c = n_r/n_o$ for "Labels" experiment with original effect estimate $\hat{\theta}_o = 0.205$ and standard error $\sigma_o = 0.051$ for uniform initial prior for effect size $\theta$ and either fixed $\tau = 0.05$ (as in main manuscript) or half normal prior with standard deviation 0.04 assigned to $\tau$. Replication success is defined by the two-trials rule at level $\alpha = 0.025$, the replication Bayes factor at level $\gamma = 1/10$, fixed effect meta-analysis at level $\alpha = 0.025^2$, effect size equivalence based on 90% confidence interval and with margin $\Delta = 0.2$, skeptical $p$-value at level $\alpha = 0.062$, and skeptical Bayes factor at level $\gamma = 1/10$.

as in the main manuscript. A half normal prior with is assigned to the heterogeneity $\tau$ which is a typical prior distribution used for heterogeneity modeling in meta-analysis (Röver et al., 2021). The standard deviation of the prior is set to 0.04 so that the mean of the prior equals the value of the fixed heterogeneity $\tau = 0.05$ elicited in the main manuscript. We see that the probability of replication success is only slightly higher compared to the fixed $\tau = 0.05$ from the main manuscript.

## 2 The two-trials rule

The two-trials rule is the most common analysis approach for replication studies. Replication success is declared if both original and replication study achieve statistical significance at some level $\alpha$ (and both estimates go in the same direction which can be taken into account by using one-sided $p$-values). We will study the two-trial under normality using the data model $\hat{\theta}_i \mid \theta \sim \mathrm{N}(\theta, \sigma_i^2)$ with $\hat{\theta}_i$ the estimate of the unknown effect size $\theta$ from study $i$ and $\sigma_i$ is the corresponding standard error (assumed to be know). The $p$-values for testing $H_0\colon \theta = 0$ versus $H_1\colon \theta > 0$ are then $p_i = 1 - \Phi(\hat{\theta}_i/\sigma_i)$ whereas for the alternative $H_1\colon \theta < 0$ they are $p_i = \Phi(\hat{\theta}_i/\sigma_i)$. Suppose the original effect estimate was statistically significant at level $\alpha$, i. e., $p_o \leq \alpha$. Replication success at level $\alpha$ is then established if the replication effect estimate $\hat{\theta}_r$ is also statistically significant at level $\alpha$, i. e., $p_r \leq \alpha$. By applying some algebraic manipulations to the success condition, one can show that this implies that replication success is achieved if the replication

effect estimate $\hat{\theta}_r$ is contained in the success region

$$S_{\text{2TR}} = \begin{cases} [z_\alpha \, \sigma_r, \infty) & \text{for } \hat{\theta}_o > 0 \\ (-\infty, -z_\alpha \, \sigma_r] & \text{for } \hat{\theta}_o < 0. \end{cases}$$

### 2.1 The multisite two-trials rule

If multiple replication studies are conducted for one original study (a *multisite* replication), the two-trials rule is typically modified by meta-analyzing the effect estimates from all replications and then using the combined estimate as usual in the two-trials rule (see e. g., the "Many labs" projects from Klein et al., 2014, 2018). Suppose $m$ replication studies are conducted and produce $m$ effect estimates $\hat{\theta}_{r1}, \dots, \hat{\theta}_m$ with standard errors $\sigma_{r1}, \dots, \sigma_{rm}$. Subsequently, a weighted average $\hat{\theta}_{r*} = \{\sum_{i=1}^m \hat{\theta}_{ri}/(\sigma_{ri}^2 + \tau_r^2)\}\, \sigma_{r*}^2$ with standard error $\sigma_{r*} = 1/\sqrt{\{\sum_i^m 1/(\sigma_{ri}^2 + \tau_r^2)\}}$ can be computed. If the between-replication heterogeneity variance $\tau_r^2$ is set to zero this corresponds to the fixed effect estimate of $\theta$, while estimating $\tau_r^2$ from the data corresponds to the random effects estimate. Replication success at level $\alpha$ is then established if the replication $p$-value is smaller than $\alpha$, i. e., $p_{r*} = 1 - \Phi(\hat{\theta}_{r*}/\sigma_{r*}) \leq \alpha$. With some algebra one can show that this implies a success region for the weighted average replication effect estimate $\hat{\theta}_{r*}$ given by

$$S_{\text{2TR}} = \begin{cases} [z_\alpha \, \sigma_{r*}, \infty) & \text{for } \hat{\theta}_o > 0 \\ (-\infty, -z_\alpha \, \sigma_{r*}] & \text{for } \hat{\theta}_o < 0. \end{cases}$$

## 3 Fixed effect meta-analysis

Assume again the data model $\hat{\theta}_i \,|\, \theta \sim \mathrm{N}(\theta, \sigma_i^2)$ where $\hat{\theta}_i$ is an estimate of the effect size $\theta$ from study $i \in \{o, r\}$ and $\sigma_i$ is the corresponding standard error (assumed to be know). In the fixed effect meta-analysis approach replicability is assessed in terms of the pooled effect estimate $\hat{\theta}_m$ and standard error $\sigma_m$ which are

$$\hat{\theta}_m = \left(\hat{\theta}_o/\sigma_o^2 + \hat{\theta}_r/\sigma_r^2\right)\sigma_m^2 \qquad \text{and} \qquad \sigma_m = \left(1/\sigma_o^2 + 1/\sigma_r^2\right)^{-1/2},$$

which are also equivalent to the mean and standard deviation of a posterior distribution for the effect size $\theta$ based on the data from original and replication study and a flat initial prior for $\theta$. Fixed effect meta-analysis is typically used because estimating a heterogeneity variance from two studies is highly unstable. Replication success at level $\alpha$ is established if the one-sided meta-analytic $p$-value (in the direction of the original effect estimate $\hat{\theta}$) is significant at level $\alpha$, i. e., $p_m = 1 - \Phi(\hat{\theta}_m/\sigma_m) \leq \alpha$ for $\hat{\theta}_o > 0$ and $p_m = \Phi(\hat{\theta}_m/\sigma_m) \leq \alpha$ for $\hat{\theta}_o < 0$. With some algebraic manipulations one can show that this criterion implies a success region $S_{\text{MA}}$ for the replication effect estimate $\hat{\theta}_r$ given by

$$S_{\text{MA}} = \begin{cases} [\sigma_r z_\alpha \sqrt{1 + \sigma_r^2/\sigma_o^2} - (\hat{\theta}_o \sigma_r^2)/\sigma_o^2, \infty) & \text{for } \hat{\theta}_o > 0 \\ (-\infty, -\sigma_r z_\alpha \sqrt{1 + \sigma_r^2/\sigma_o^2} - (\hat{\theta}_o \sigma_r^2)/\sigma_o^2] & \text{for } \hat{\theta}_o < 0. \end{cases}$$

## 4 Effect size equivalence

The effect size equivalence approach (Anderson and Maxwell, 2016) defines replication success via compatibility of the effect estimates from both studies. Under normality we may assume the data model

$\hat{\theta}_i \mid \theta_i \sim \mathrm{N}(\theta_i, \sigma_i^2)$ for study $i \in \{o, r\}$, and we are interested in the true effect size difference $\delta = \theta_r - \theta_o$. A $(1-\alpha)$ confidence interval for $\delta$ is then given by

$$C_\alpha = \left[\hat{\theta}_r - \hat{\theta}_o - z_{\alpha/2}\sqrt{\sigma_r^2 + \sigma_r^2}, \hat{\theta}_r - \hat{\theta}_o + z_{\alpha/2}\sqrt{\sigma_r^2 + \sigma_r^2}\right]$$

Effect size equivalence is established if the confidence interval is fully included in an equivalence region $C_\alpha \subseteq [-\Delta, \Delta]$ with $\Delta > 0$ a pre-specified margin. Applying some algebraic manipulations to the success conditions one can show that the equivalence test replication success criterion implies a success region $S_{\mathrm{E}}$ for the replication estimate $\hat{\theta}_r$ given by

$$S_{\mathrm{E}} = \left[\hat{\theta}_o - \Delta + z_{\alpha/2}\sqrt{\sigma_o^2 + \sigma_r^2}, \hat{\theta}_o + \Delta - z_{\alpha/2}\sqrt{\sigma_o^2 + \sigma_r^2}\right].$$

# 5 The replication Bayes factor

The replication Bayes factor approach uses the replication data $x_r$ to quantify the evidence for the null hypothesis $H_0\colon \theta = 0$ relative to the alternative hypothesis $H_1\colon \theta \sim f(\theta \mid x_o)$, which postulates that the effect size $\theta$ is distributed according to its posterior distribution based on the original data $x_o$. Assume again a normal model $\hat{\theta}_i \mid \theta \sim \mathrm{N}(\theta, \sigma_i^2)$ with $\hat{\theta}_i$ an estimate of the effect size $\theta$ from study $i \in \{o, r\}$ and $\sigma_i$ the corresponding standard error (assumed to be know), and that we use the alternative $H_1\colon \theta \sim \mathrm{N}(\hat{\theta}_o, \sigma_o^2)$ which arises from updating a flat initial prior for $\theta$ the original data $x_o = \{\hat{\theta}_o, \sigma_o\}$. The replication Bayes factor is then

$$\mathrm{BF}_{\mathrm{R}} = \frac{f(\hat{\theta}_r \mid H_0)}{f(\hat{\theta}_r \mid H_1)} = \sqrt{1 + \sigma_o^2/\sigma_r^2}\,\exp\left[-\frac{1}{2}\left\{\frac{\hat{\theta}_r^2}{\sigma_r^2} - \frac{(\hat{\theta}_r - \hat{\theta}_o)^2}{\sigma_o^2 + \sigma_r^2}\right\}\right]. \quad (1)$$

Replication success at level $\gamma \in (0, 1)$ is achieved if $\mathrm{BF}_{\mathrm{R}} \leq \gamma$. By applying some algebra to $\mathrm{BF}_{\mathrm{R}} \leq \gamma$, one can show that it is equivalent to the replication effect estimate $\hat{\theta}_r$ falling in the success region

$$S_{\mathrm{BF}_{\mathrm{R}}} = \left(-\infty, -\sqrt{A} - (\hat{\theta}_o\sigma_r^2)/\sigma_o^2\right] \bigcup \left[\sqrt{A} - (\hat{\theta}_o\sigma_r^2)/\sigma_o^2, \infty\right)$$

where $A = \sigma_r^2(1 + \sigma_r^2/\sigma_o^2)\{\hat{\theta}_o^2/\sigma_o^2 - 2\log\gamma + \log(1 + \sigma_o^2/\sigma_r^2)\}$.

## 5.1 The multisite replication Bayes factor

The generalization of the replication Bayes factor to the multisite setting is straightforward. The data are represented by vector of replication effect estimates $\hat{\boldsymbol{\theta}}_r = (\hat{\theta}_{r1}, \dots, \hat{\theta}_{rm})^\top$ with corresponding standard error vector $\boldsymbol{\sigma}_r = (\sigma_{r1}, \dots, \sigma_{rm})^\top$, and we assume the data model $\hat{\boldsymbol{\theta}}_r \mid \theta \sim \mathrm{N}_m\{\theta\,\mathbf{1}_m, \mathrm{diag}(\boldsymbol{\sigma}^2 + \tau_r^2\,\mathbf{1}_m\}$ where $\mathbf{1}_m$ is a vector of $m$ ones and $\tau_r^2$ is a heterogeneity variance for the replication effect sizes (not to be confused with the heterogeneity variance $\tau^2$ used in the design prior).

As in the singlesite case, the replication Bayes factor quantifies the evidence that the data provide for the null hypothesis $H_0\colon \theta = 0$ relative to the alternative hypothesis $H_1\colon \theta \sim \mathrm{N}(\hat{\theta}_o, \sigma_o^2)$. The marginal density of the replication data under the null hypothesis is simply $\hat{\boldsymbol{\theta}}_r \mid H_0 \sim \mathrm{N}_m\{0\,\mathbf{1}_m, \mathrm{diag}(\boldsymbol{\sigma}^2 + \tau_r^2\,\mathbf{1}_m\}$, whereas the marginal likelihood under the alternative $H_1$ is obtained from integrating the likelihood with respect to the prior distribution of $\theta$ under the alternative $H_1$. Let $\mathrm{N}(x; m, v)$ denote the normal density function mean $m$ and variance $v$ evaluated at $x$. Define also $\hat{\theta}_{r*} = \left\{\sum_{i=1}^n \hat{\theta}_{ri}/(\sigma_{ri}^2 + \tau_r^2)\right\}\sigma_{r*}^2$ and $\sigma_{r*}^2 = 1/\left\{\sum_{i=1}^n 1/(\sigma_{ri}^2 + \tau_r^2)\right\}$, i.e., the weighted average of the replication effect estimates based

on the heterogeneity $\tau_r^2$ and its variance. The marginal density is then

$$
\begin{aligned}
f(\hat{\boldsymbol{\theta}}_r \mid H_1) &= \int f(\hat{\boldsymbol{\theta}}_r \mid \theta) f(\theta \mid H_1)\, \mathrm{d}\theta \\
&= \int \frac{\exp\left[-\frac{1}{2}\left\{\sum_{i=1}^n \frac{(\hat{\theta}_{ri}-\theta)^2}{\sigma_{ri}^2+\tau_r^2} + \frac{(\theta-\hat{\theta}_o)^2}{\sigma_o^2}\right\}\right]}{\left\{2\pi\sigma_o^2 \prod_{i=1}^n 2\pi\left(\sigma_{ri}^2+\tau_r^2\right)\right\}^{1/2}}\, \mathrm{d}\theta \\
&= \int \frac{\exp\left[-\frac{1}{2}\left\{\sum_{i=1}^n \frac{(\hat{\theta}_{ri}-\hat{\theta}_{r*})^2}{\sigma_{ri}^2+\tau_r^2} + \frac{(\hat{\theta}_{r*}-\theta)^2}{\sigma_{r*}^2} + \frac{(\theta-\hat{\theta}_o)^2}{\sigma_o^2}\right\}\right]}{\left\{2\pi\sigma_o^2 \prod_{i=1}^n 2\pi\left(\sigma_{ri}^2+\tau_r^2\right)\right\}^{1/2}}\, \mathrm{d}\theta \\
&= \frac{\exp\left[-\frac{1}{2}\left\{\sum_{i=1}^n \frac{(\hat{\theta}_{ri}-\hat{\theta}_{r*})^2}{\sigma_{ri}^2+\tau_r^2}\right\}\right]}{\left\{2\pi\sigma_o^2 \prod_{i=1}^n 2\pi\left(\sigma_{ri}^2+\tau_r^2\right)\right\}^{1/2}} \underbrace{\int \exp\left[-\frac{1}{2}\left\{\frac{(\hat{\theta}_{r*}-\theta)^2}{\sigma_{r*}^2} + \frac{(\theta-\hat{\theta}_o)^2}{\sigma_o^2}\right\}\right] \mathrm{d}\theta}_{=\mathrm{N}(\hat{\theta}_{r*};m,\sigma_o^2+\sigma_{r*}^2)2\pi\sigma_o\sigma_{r*}} \\
&= \left\{(1+\sigma_o^2/\sigma_{r*}^2)\prod_{i=1}^n 2\pi\left(\sigma_{ri}^2+\tau_r^2\right)\right\}^{-1/2} \exp\left[-\frac{1}{2}\left\{\sum_{i=1}^n \frac{(\hat{\theta}_{ri}-\hat{\theta}_{r*})^2}{\sigma_{ri}^2+\tau_r^2} + \frac{(\hat{\theta}_{r*}-\hat{\theta}_o)^2}{\sigma_{r*}^2+\sigma_o^2}\right\}\right].
\end{aligned}
$$

Dividing the marginal density of $\hat{\boldsymbol{\theta}}_r$ under $H_0$ by the marginal density of $\hat{\boldsymbol{\theta}}_r$ under $H_1$ leads to cancellation of several terms, and produces the replication Bayes factor

$$
\mathrm{BF}_{01}(\hat{\boldsymbol{\theta}}_r) = \frac{f(\hat{\boldsymbol{\theta}}_r \mid H_0)}{f(\hat{\boldsymbol{\theta}}_r \mid H_1)} = \sqrt{1+\sigma_o^2/\sigma_{r*}^2}\, \exp\left[-\frac{1}{2}\left\{\frac{\hat{\theta}_{r*}^2}{\sigma_{r*}^2} - \frac{(\hat{\theta}_{r*}-\hat{\theta}_o)^2}{\sigma_{r*}^2+\sigma_o^2}\right\}\right].
$$

The multisite replication Bayes factor is therefore equivalent to the singlesite replication Bayes factor from (1) but using the weighted average $\hat{\theta}_{r*}$ and its standard error $\sigma_{r*}$ as the replication effect estimate $\hat{\theta}_r$ and standard error $\sigma_r$.

## 6 The skeptical *p*-value

Held (2020) proposed a reverse-Bayes approach for assessing replicability. One assumes again the data model $\hat{\theta}_i \mid \theta \sim \mathrm{N}(\theta, \sigma_i^2)$ with $i \in \{o, r\}$, along with a zero-mean "skeptical" prior $\theta \sim \mathrm{N}(0, \sigma_s^2)$ for the effect size. In a first step, a level $\alpha \geq p_o = 1 - \Phi(|\hat{\theta}_o|/\sigma_o)$ is fixed and the "sufficiently skeptical" prior variance $\sigma_s^2$ is computed

$$
\sigma_s^2 = \frac{\sigma_o^2}{(z_o^2/z_\alpha^2) - 1}
$$

where $z_o = \hat{\theta}_o/\sigma_o$. The sufficiently skeptical prior variance $\sigma_s^2$ has the property that it renders the resulting posterior of $\theta$ no longer "credible" at level $\alpha$, that is, the posterior tail probability is fixed to $\Pr(\theta \geq 0 \mid \hat{\theta}_o, \sigma_o, \sigma_s) = 1 - \alpha$ for positive estimates and $\Pr(\theta \leq 0 \mid \hat{\theta}_o, \sigma_o, \sigma_s) = 1 - \alpha$ for negative estimates. In a second step, the conflict between the skeptical prior and the observed replication data is quantified, larger conflict indicating a higher degree of replication success. For doing so, a prior predictive tail probability

$$
p_{\text{Box}} = \begin{cases} 1 - \Phi\left\{\hat{\theta}_r/(\sigma_r^2+\sigma_s^2)\right\} & \text{if } \hat{\theta}_o > 0 \\ \Phi\left\{\hat{\theta}_r/(\sigma_r^2+\sigma_s^2)\right\} & \text{if } \hat{\theta}_o < 0 \end{cases}
$$

is computed and replication success at level $\alpha$ is declared if $p_{\text{Box}} \leq \alpha$. The smallest level $\alpha$ at which replication success is achieved is called the *the skeptical p-value* $p_{\text{S}}$ and replication success at level $\alpha$ is equivalent with $p_{\text{S}} \leq \alpha$ (see Held, 2020; Held et al., 2022, for more details on $p_{\text{S}}$). By applying some algebraic manipulations to the condition $p_{\text{Box}} \leq \alpha$, one can show that it is equivalent to the replication effect estimate $\hat{\theta}_r$ falling in the success region

$$S_{p_{\text{S}}} = \begin{cases} [z_\alpha \sqrt{\{\sigma_r^2 + \frac{\sigma_o^2}{(z_o^2/z_\alpha^2)-1}\}}, \infty) & \text{if } \hat{\theta}_o > 0 \\ (-\infty, -z_\alpha \sqrt{\{\sigma_r^2 + \frac{\sigma_o^2}{(z_o^2/z_\alpha^2)-1}\}}] & \text{if } \hat{\theta}_o < 0. \end{cases}$$

## 7 The skeptical Bayes factor

Pawel and Held (2022) modified the reverse-Bayes assessment of replication success from Held (2020) to use Bayes factors (Jeffreys, 1961; Kass and Raftery, 1995) instead of tail probabilities as measures of evidence and prior data conflict. The procedure assumes again the data model $\hat{\theta}_i \mid \theta \sim \text{N}(\theta, \sigma_i^2)$ for study $i \in \{o, r\}$. In the first step the original data are used to contrast the evidence for the point null hypothesis $H_0\colon \theta = 0$ relative to the "skeptical" alternative $H_S\colon \theta \sim \text{N}(0, \sigma_s^2)$ with the Bayes factor

$$\text{BF}_{0S} = \frac{f(\hat{\theta}_o \mid H_0)}{f(\hat{\theta}_o \mid H_S)} = \sqrt{1 + \sigma_s^2/\sigma_o^2} \exp\left\{-\frac{z_o^2}{2(1 + \sigma_o^2/\sigma_s^2)}\right\}.$$

where $z_o = \hat{\theta}_o/\sigma_o$. One then determines the sufficiently skeptical prior variance $\sigma_s^2$ so that the Bayes factor is fixed to a level $\gamma \in (0, 1)$ meaning that there is no longer evidence against the null hypothesis at level $\gamma$. The sufficiently skeptical prior variance can be computed by

$$\sigma_s^2 = \begin{cases} -\dfrac{\hat{\theta}_o^2}{q} - \sigma_o^2 & \text{if } -\dfrac{\hat{\theta}_o^2}{q} \geq \sigma_o^2 \\ \text{undefined} & \text{else} \end{cases} \tag{2}$$

$$\text{where } q = \text{W}_{-1}\left\{-\frac{z_o^2}{\gamma^2} \exp\left(-z_o^2\right)\right\} \tag{3}$$

with $\text{W}_{-1}(\cdot)$ the branch of the Lambert W function with $\text{W}(y) \leq -1$ for $y \in [-1/e, 0)$.

In a second step the conflict between the skeptical prior and the replication data is quantified. To do so, the skeptic is contrasted to the "advocacy" alternative $H_A\colon \theta \sim \text{N}(\hat{\theta}_o, \sigma_o^2)$ which represents the position of an advocate as the prior corresponds to the posterior distribution based on the original data $\{\hat{\theta}_o, \sigma_o\}$ and a flat prior for the effect size $\theta$. This is done by computing the Bayes factor

$$\text{BF}_{SA} = \frac{f(\hat{\theta}_r \mid H_S)}{f(\hat{\theta}_r \mid H_A)} = \sqrt{\frac{\sigma_o^2 + \sigma_r^2}{\sigma_s^2 + \sigma_r^2}} \exp\left[-\frac{1}{2}\left\{\frac{\hat{\theta}_r^2}{\sigma_s^2 + \sigma_r^2} - \frac{(\hat{\theta}_r - \hat{\theta}_o^2)}{\sigma_o^2 + \sigma_r^2}\right\}\right]$$

and replication success at level $\gamma$ is defined by $\text{BF}_{SA} \leq \gamma$ as the data favor the advocate over the skeptic at a higher level than the skeptic's initial objection to the null hypothesis. The smallest level $\gamma$ at which replication success is achievable is then called *the skeptical Bayes factor* $\text{BF}_{\text{S}}$, and replication success at level $\gamma$ is equivalent to $\text{BF}_{\text{S}} \leq \gamma$ (see Pawel and Held, 2022, for details on how to compute $\text{BF}_{\text{S}}$). To derive the success region of the skeptical Bayes factor one can apply algebraic manipulations to $\text{BF}_{SA} \leq \gamma$, the

condition for replication success at level $\gamma$, which leads to

$$S_{\text{BF}_{\text{S}}} = \begin{cases} (-\infty, -\sqrt{B} - M] \bigcup [\sqrt{B} - M, \infty) & \text{for } \sigma_s^2 < \sigma_o^2 \\ [\hat{\theta}_o - \{(\sigma_o^2 + \sigma_r^2) \log \gamma\}/\hat{\theta}_o, \infty) & \text{for } \sigma_s^2 = \sigma_o^2 \\ [-\sqrt{B} - M, \sqrt{B} - M] & \text{for } \sigma_s^2 > \sigma_o^2 \end{cases} \tag{4}$$

with

$$B = \left\{ \frac{\hat{\theta}_o^2}{\sigma_o^2 - \sigma_s^2} + 2 \log \left( \frac{\sigma_o^2 + \sigma_r^2}{\sigma_s^2 + \sigma_r^2} \right) - 2 \log \gamma \right\} \frac{(\sigma_s^2 + \sigma_r^2)(\sigma_o^2 + \sigma_r^2)}{\sigma_o^2 - \sigma_s^2}$$

$$M = \frac{\hat{\theta}_o(\sigma_s^2 + \sigma_r^2)}{\sigma_o^2 - \sigma_s^2}$$

and the sufficiently skeptical prior variance $\sigma_s^2$ computed by (2).

## 8 Optimal number of sites

The total cost of the design are $K = m(K_c n_r + K_s)$ so that we can write the number of sites $m$ for a given total cost as

$$m = K(K_c n_r + K_s)^{-1}. \tag{5}$$

We now want to minimize the predictive variance of the weighted average $\hat{\theta}_{r*}$ which, for a balanced design, is given by

$$\sigma^2_{\hat{\theta}_{r*}} = \frac{\sigma_r^2 + \tau^2}{m} + \frac{\tau^2 + \sigma_o^2}{1 + 1/g}. \tag{6}$$

Plugging in (5) into (6) and minimizing it with respect to $n_r$, leads to the optimal sample size

$$n_r^* = \frac{\lambda}{\tau} \sqrt{\frac{K_s}{K_c}}$$

for a given cost ratio $K_s/K_c$.

## 9 Sample size determination for all studies from the replication project

Figure 3 shows SSD for all studies from the Protzko et al. (2020) replication project using a flat prior for the effect size $\theta$. As for the illustrative subset in the main manuscript, for the majority of studies all methods except the equivalence test require fewer samples in the replication than in the original study.

Figure 4 shows the same analyses but using an "adaptive shrinkage prior" for $\theta$ (i.e., the variance of the shrinkage prior is estimated by empirical Bayes). We see that the required sample size increases for studies with large $p$-values compared to the analysis based on a flat prior for $\theta$, whereas it stays roughly the same for studies with small $p$-values. This is because studies with large $p$-values receive more shrinkage while the shrinkage disappears with decreasing $p$-value (Pawel and Held, 2020).

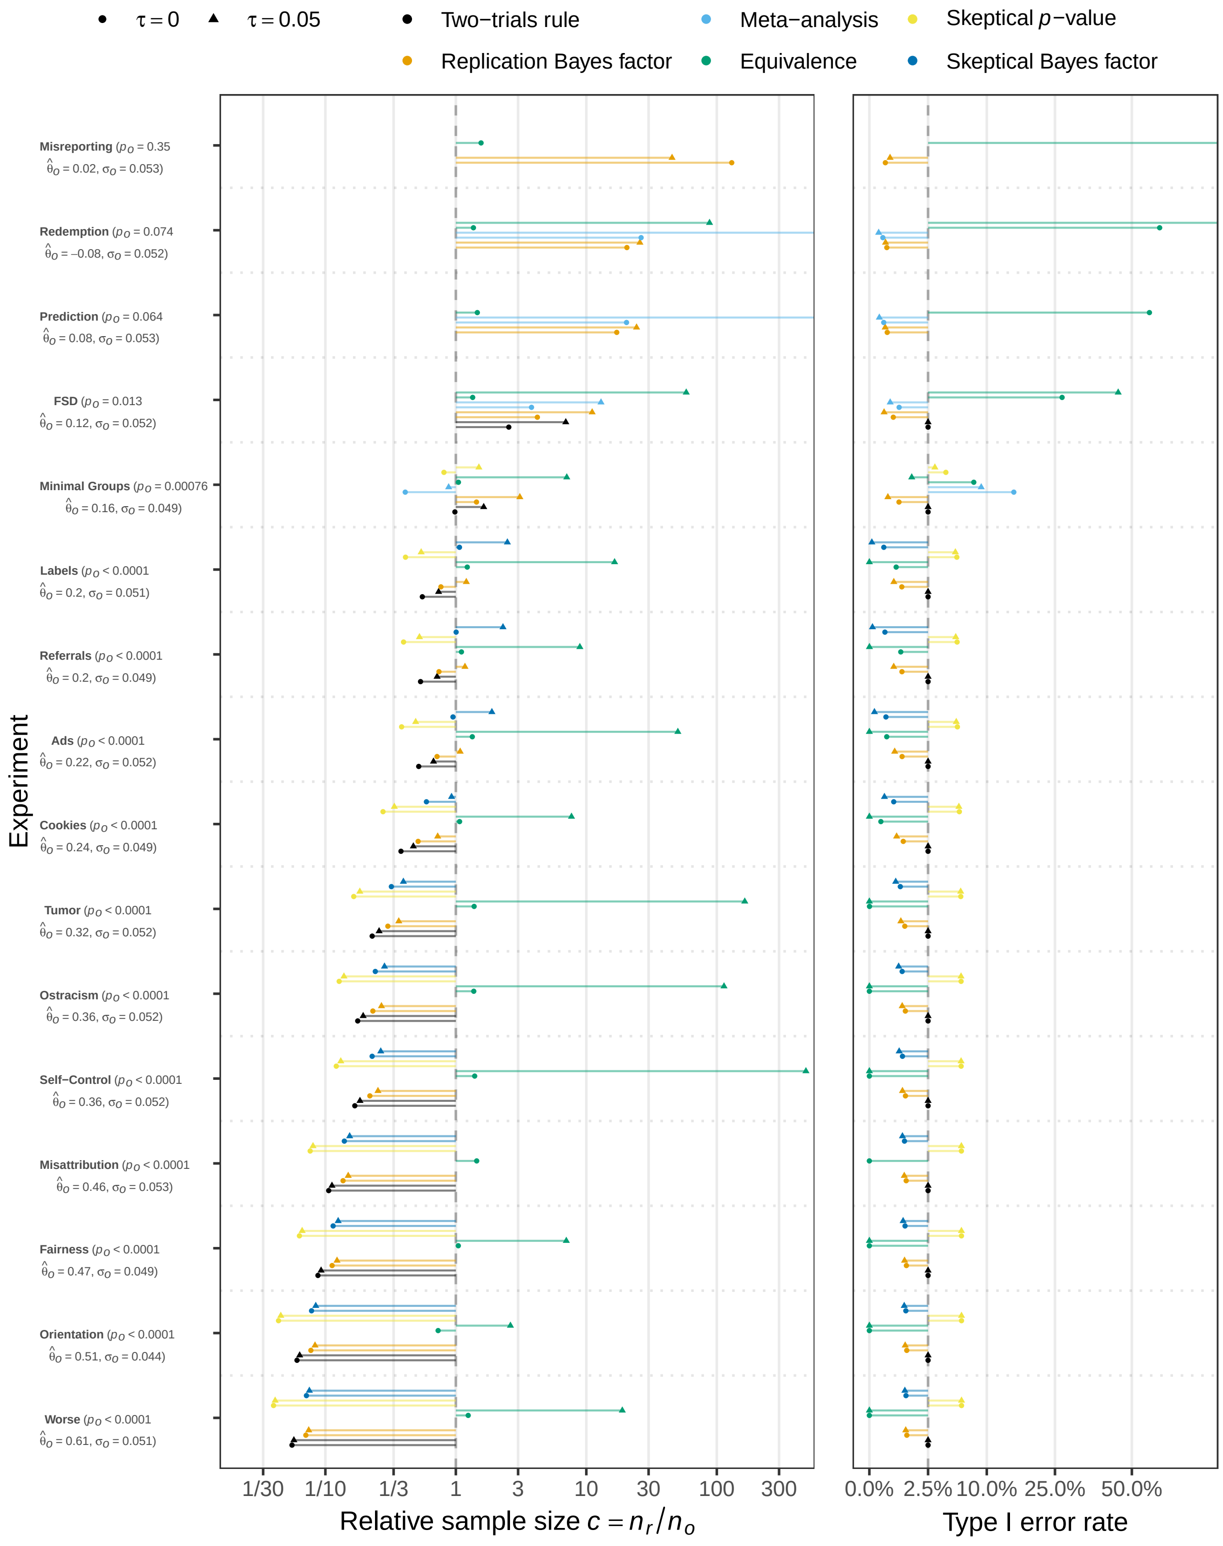


**Figure 3:** The left plot shows the required relative sample size $c = n_r/n_o$ to achieve a target probability of replication success of $1 - \beta = 80\%$ (if possible). Replication success is defined through the two-trials rule at level $\alpha = 0.025$, replication Bayes factor at level $\gamma = 1/10$, fixed effect meta-analysis at level $\alpha = 0.025^2$, effect size equivalence at level $\alpha = 0.1$ with margin $\Delta = 0.2$, skeptical $p$-value at level $\alpha = 0.062$, and skeptical Bayes factor at level $\gamma = 1/10$ for data from the replication project by Protzko et al. (2020). A flat initial prior ($\mu_\theta = 0, \sigma^2_\theta \to \infty$) is used for the effect size $\theta$ is used either without ($\tau = 0$) or with heterogeneity ($\tau = 0.05$). The right plot shows the type I error rate associated with the required sample size. Experiments are ordered (top to bottom) by their original one-sided $p$-value $p_o = 1 - \Phi(|\hat{\theta}_o|/\sigma_o)$.

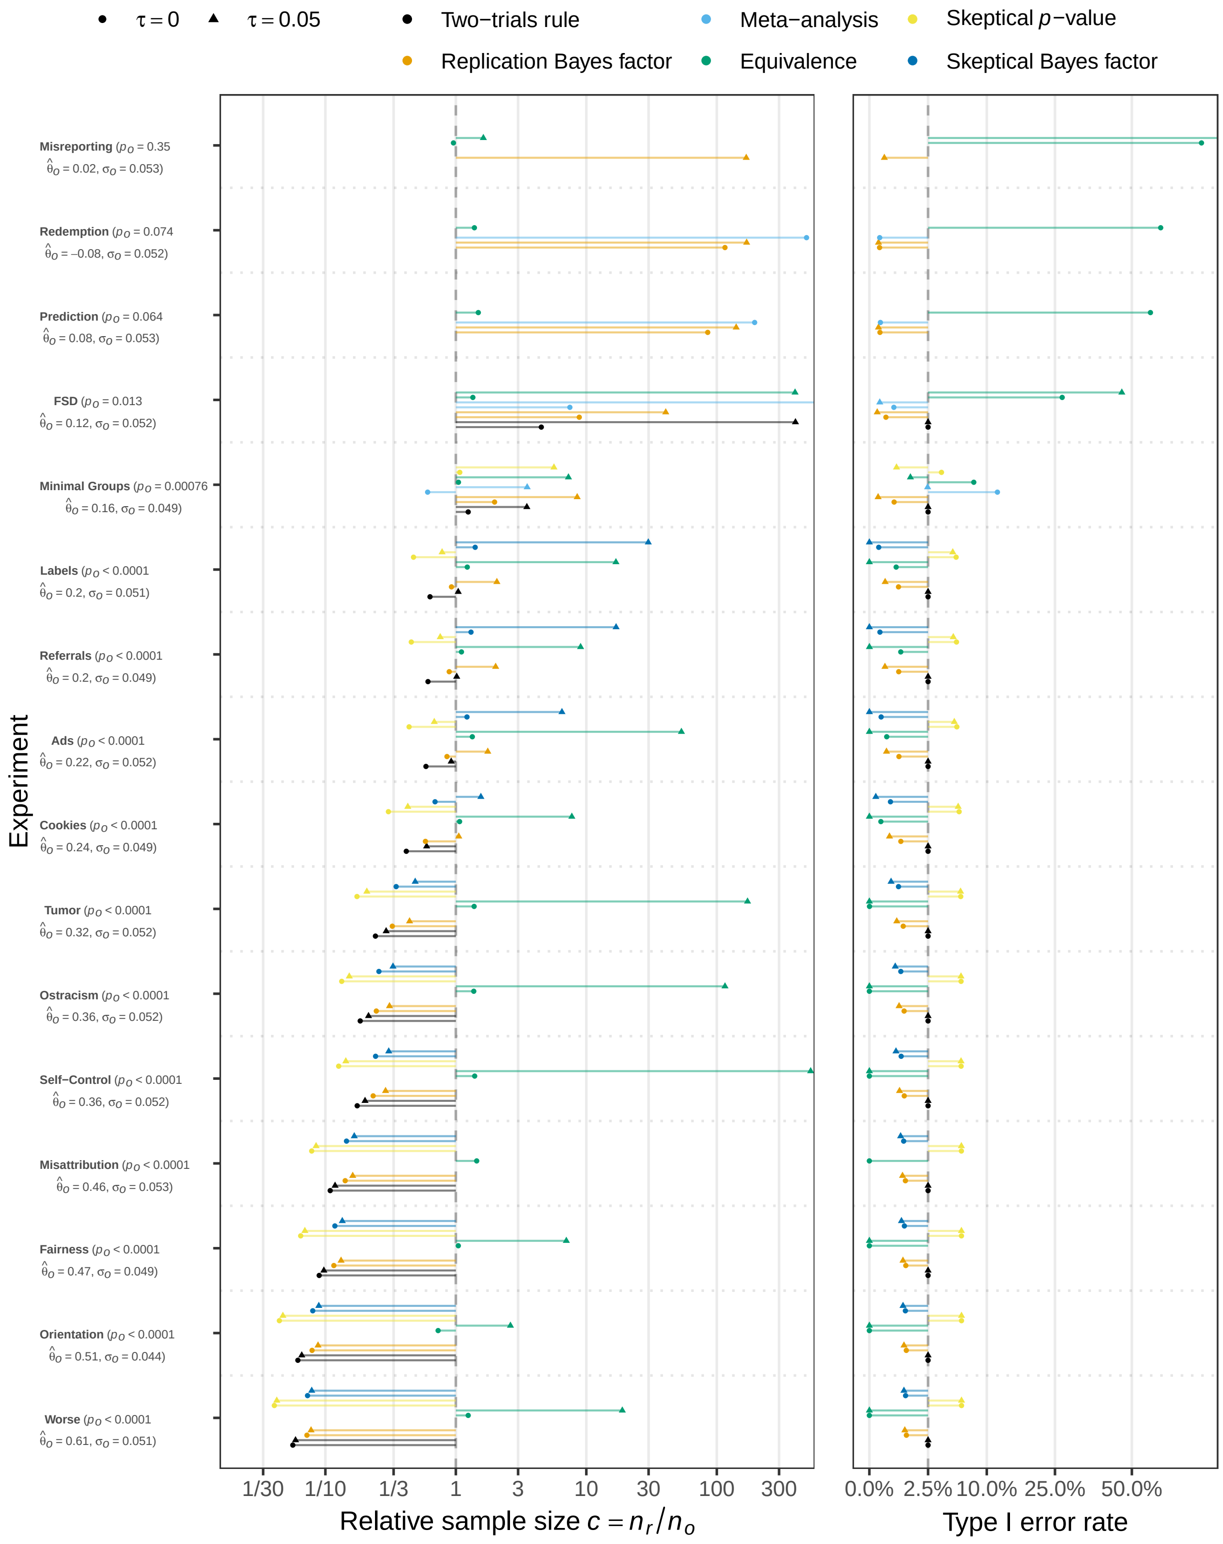


**Figure 4:** The left plot shows the required relative sample size $c = n_r/n_o$ to achieve a target probability of replication success of $1 - \beta = 80\%$ (if possible). Replication success is defined through the two-trials rule at level $\alpha = 0.025$, replication Bayes factor at level $\gamma = 1/10$, fixed effect meta-analysis at level $\alpha = 0.025^2$, effect size equivalence at level $\alpha = 0.1$ with margin $\Delta = 0.2$, skeptical $p$-value at level $\alpha = 0.062$, and skeptical Bayes factor at level $\gamma = 1/10$ for data from the replication project by Protzko et al. (2020). An adaptive shrinkage prior is used for the effect size $\theta$ either without ($\tau = 0$) or with between-study heterogeneity ($\tau = 0.05$). The right plot shows the type I error rate associated with the required sample size. Experiments are ordered (top to bottom) by their original one-sided $p$-value $p_o = 1 - \Phi(|\hat{\theta}_o|/\sigma_o)$.

## References

Anderson, S. F. and Maxwell, S. E. (2016). There's more than one way to conduct a replication study: Beyond statistical significance. *Psychological Methods*, 21(1):1–12. doi:10.1037/met0000051.

Held, L. (2020). A new standard for the analysis and design of replication studies (with discussion). *Journal of the Royal Statistical Society: Series A (Statistics in Society)*, 183(2):431–448. doi:10.1111/rssa.12493.

Held, L., Micheloud, C., and Pawel, S. (2022). The assessment of replication success based on relative effect size. *The Annals of Applied Statistics*, 16(2):706–720. doi:10.1214/21-aoas1502.

Jeffreys, H. (1961). *Theory of Probability*. Oxford: Clarendon Press, third edition.

Kass, R. E. and Raftery, A. E. (1995). Bayes factors. *Journal of the American Statistical Association*, 90(430):773–795. doi:10.1080/01621459.1995.10476572.

Klein, R. A., Ratliff, K. A., Vianello, M., Adams, R. B., Bahník, v., Bernstein, M. J., Bocian, K., Brandt, M. J., Brooks, B., et al. (2014). Investigating variation in replicability: A "many labs" replication project. *Social Psychology*, 45(3):142–152. doi:10.1027/1864-9335/a000178.

Klein, R. A., Vianello, M., Hasselman, F., Adams, B. G., Reginald B. Adams, J., Alper, S., Aveyard, M., Axt, J. R., Babalola, M. T., et al. (2018). Many labs 2: Investigating variation in replicability across samples and settings. *Advances in Methods and Practices in Psychological Science*, 1(4):443–490. doi:10.1177/2515245918810225.

Pawel, S. and Held, L. (2020). Probabilistic forecasting of replication studies. *PLOS ONE*, 15(4):e0231416. doi:10.1371/journal.pone.0231416.

Pawel, S. and Held, L. (2022). The sceptical Bayes factor for the assessment of replication success. *Journal of the Royal Statistical Society: Series B (Statistical Methodology)*, 84(3):879–911. doi:10.1111/rssb.12491.

Protzko, J., Krosnick, J., Nelson, L. D., Nosek, B. A., Axt, J., Berent, M., Buttrick, N., DeBell, M., Ebersole, C. R., Lundmark, S., MacInnis, B., O'Donnell, M., Perfecto, H., Pustejovsky, J. E., Roeder, S. S., Walleczek, J., and Schooler, J. (2020). High replicability of newly-discovered social-behavioral findings is achievable. doi:10.31234/osf.io/n2a9x. Preprint.

Röver, C., Bender, R., Dias, S., Schmid, C. H., Schmidli, H., Sturtz, S., Weber, S., and Friede, T. (2021). On weakly informative prior distributions for the heterogeneity parameter in Bayesian random-effects meta-analysis. *Research Synthesis Methods*, 12(4):448–474. doi:10.1002/jrsm.1475.
